# Supplementary material for: MONAS: Multi-Objective Neural Architecture Search using Reinforcement Learning
Source: arXiv:1806.10332 source file (2018-12-03)
Supplement: Supplementary file 2 [file 07AppendixB.tex]

\begin{figure}[h]
\centering
\subfigure[$\alpha=0.25$]
{\includegraphics[width=0.45\textwidth]{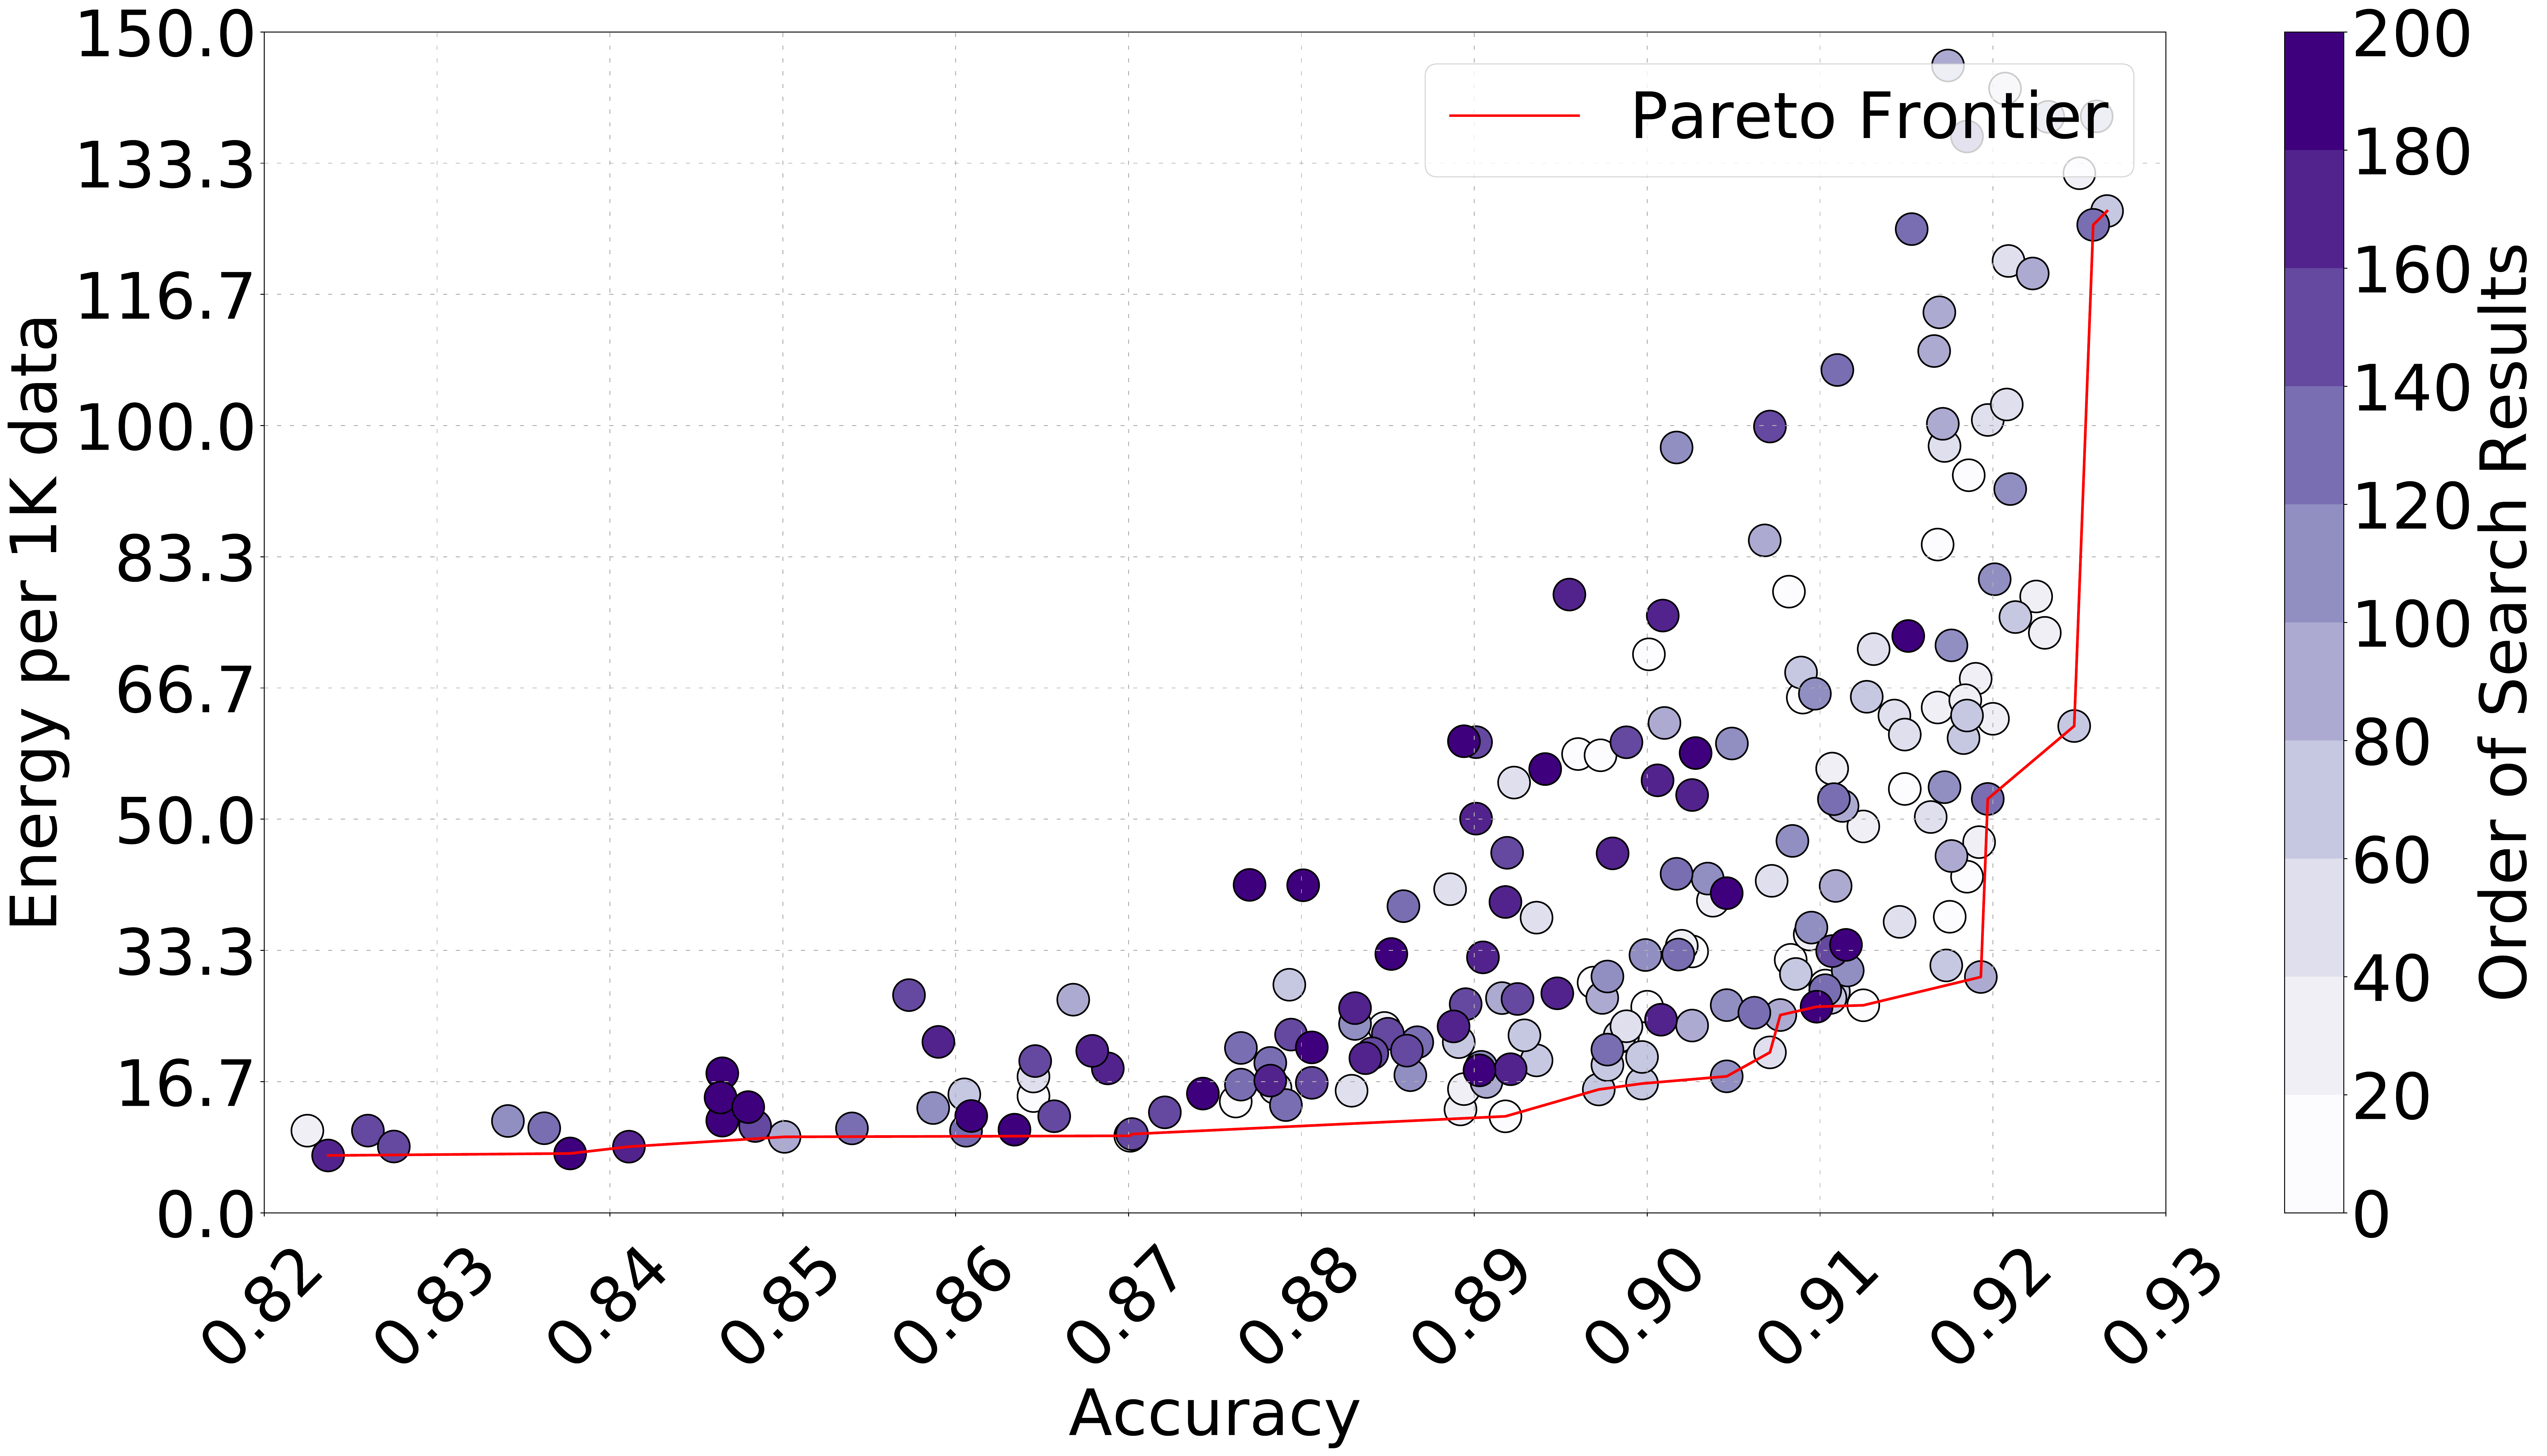}
\label{fig:condensenet_0.25}}
\subfigure[$\alpha=0.75$]
{\includegraphics[width=0.45\textwidth]{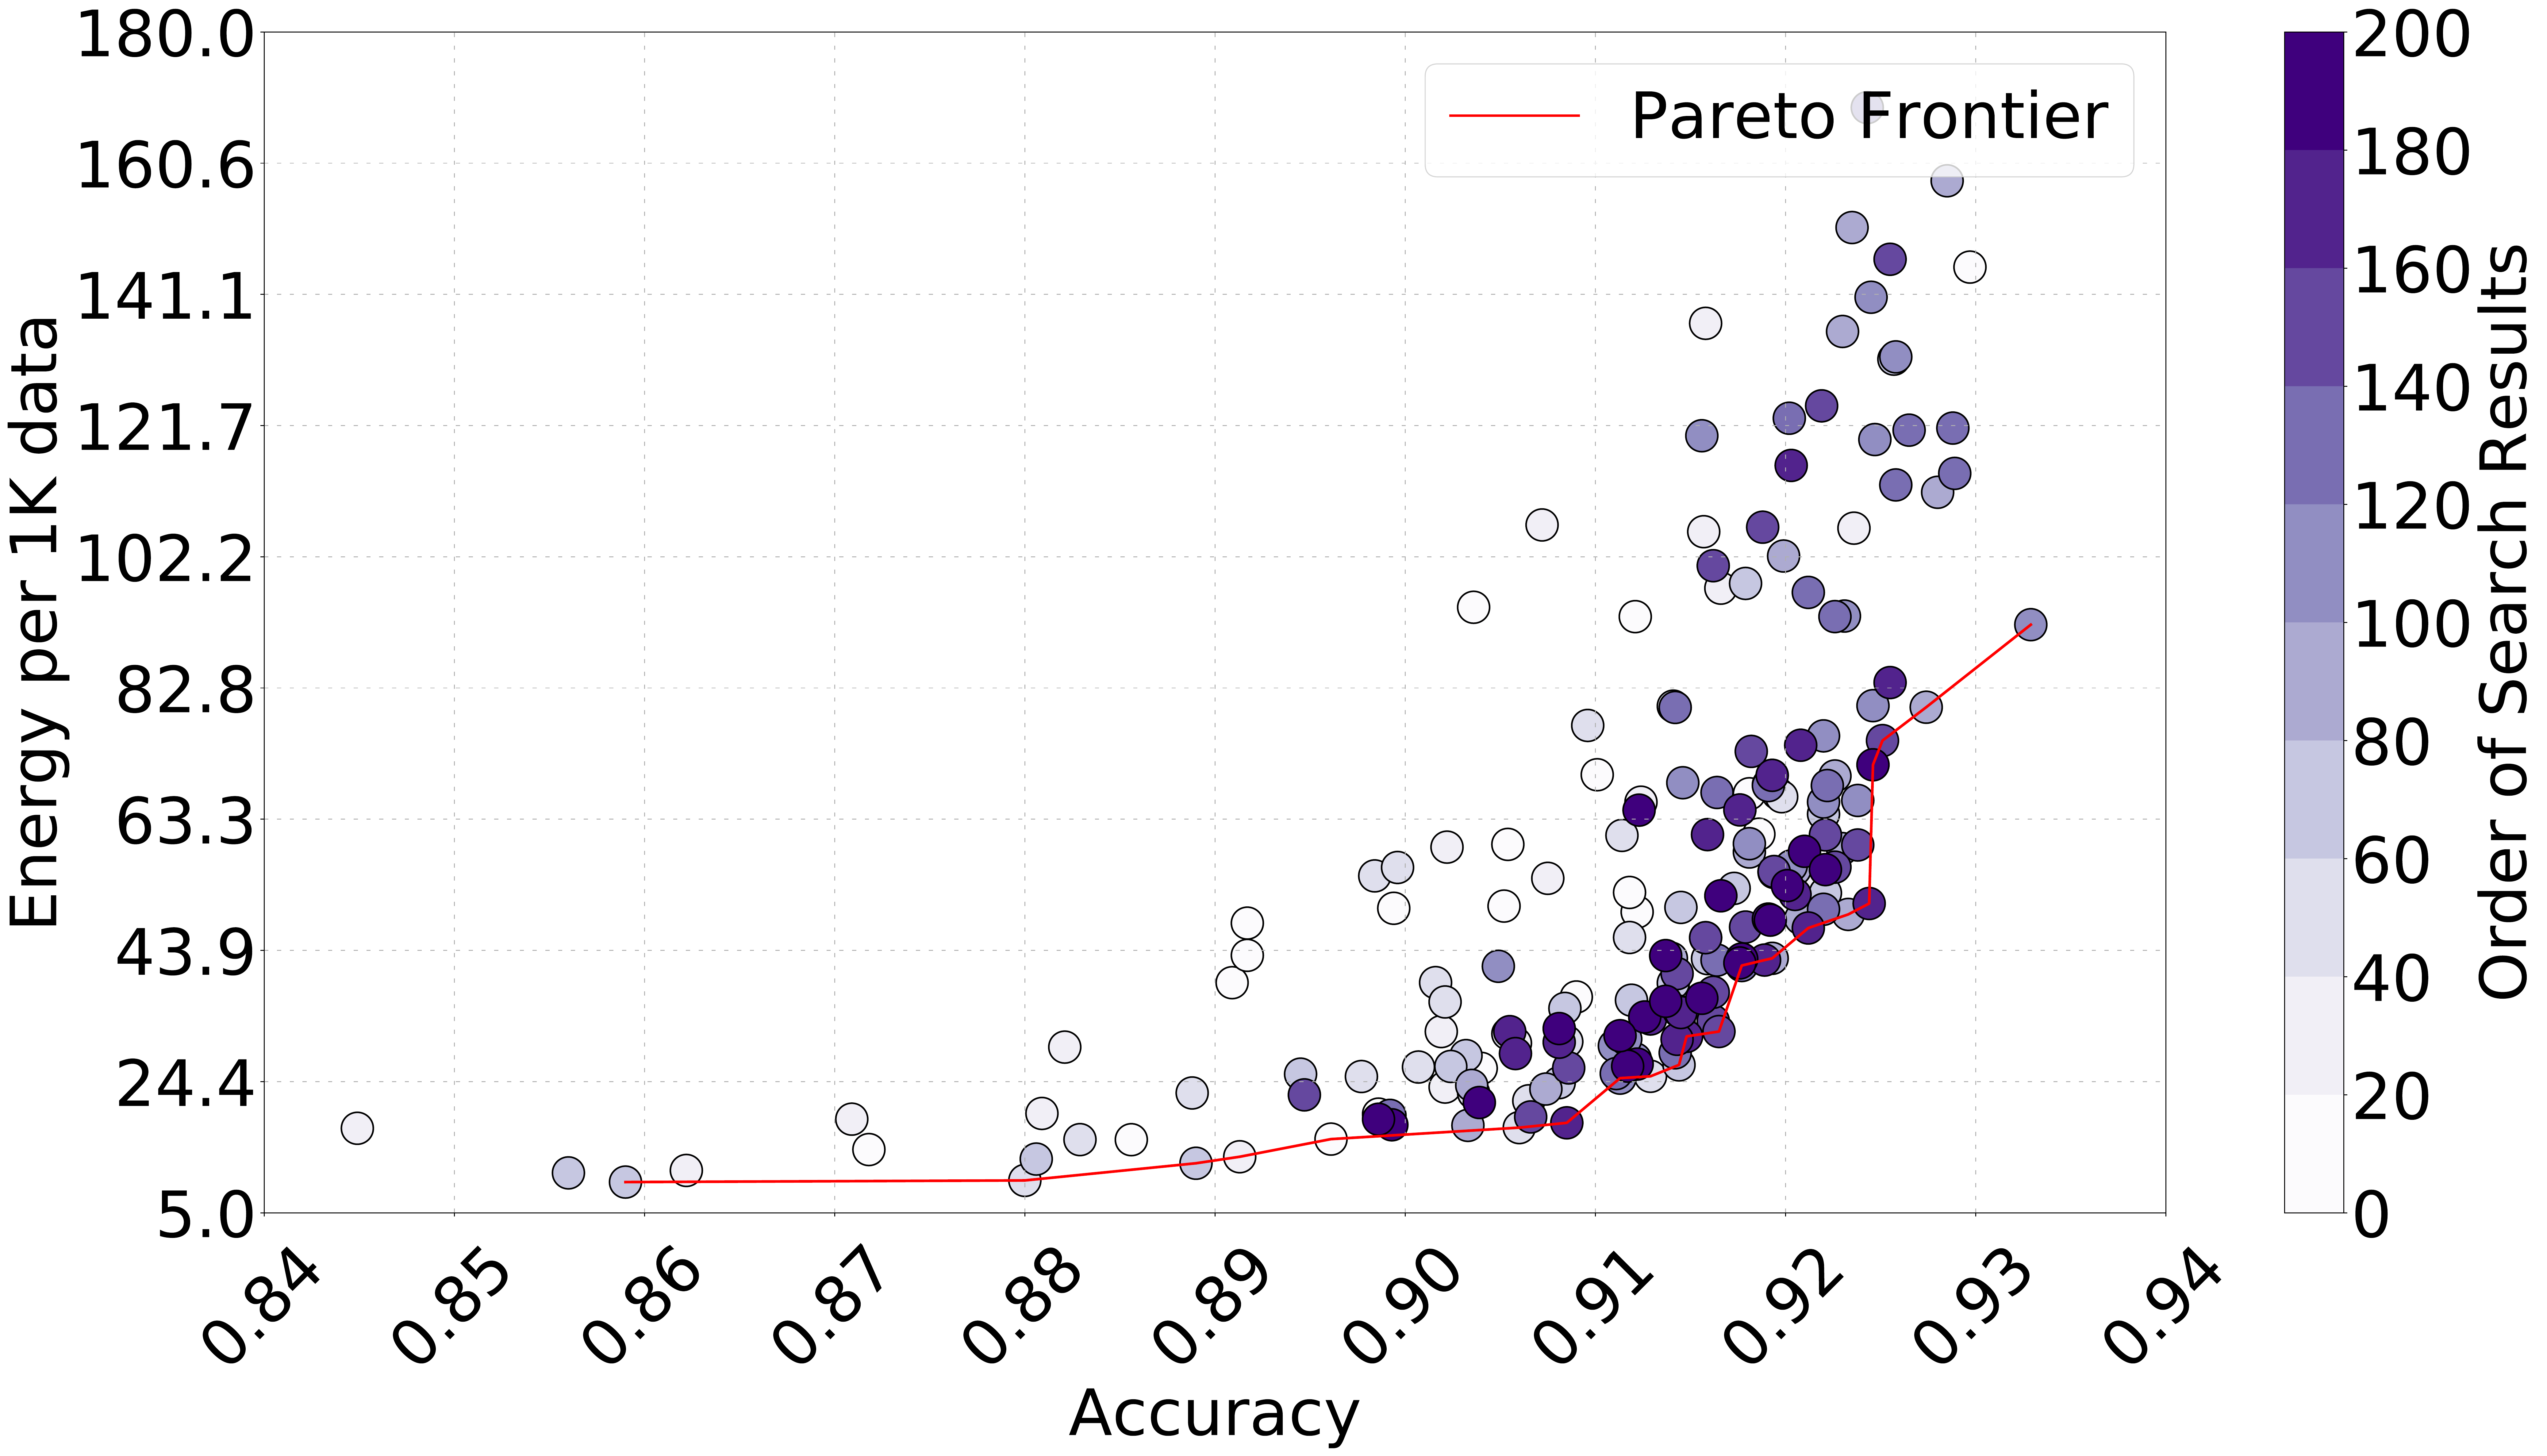}
\label{fig:condensenet_0.75}}
\caption{Applying different $\alpha$ when searching CondenseNet}
\label{fig:condensenet_mix}
\end{figure}

\end{figure}

\begin{table*}[h]
  \begin{center}
    \begin{tabular}{|c|c|c|c|c|c|c|c|c|} 
    \hline
%       \textbf{Model} & \textbf{FN1} & \textbf{FH1} & \textbf{FW1} & \textbf{FN2} & \textbf{FH2} & \textbf{FW2} & \textbf{Error(\%)} & \textbf{Energy(J)} \\
%       \hline 
%       \multirow{3}{*}{AlexNet} 
%       & 64 & 5 & 9 & 64 & 5 & 5 & 13.5 & 4.197\\
%       & 64 & 5 & 5 & 64 & 5 & 5 & 13.6 & 3.802\\
%       & 64 & 3 & 5 & 64 & 5 & 5 & 13.7 & 3.796\\
%       \hline
%       \hline
      \textbf{Model} & \textbf{ST1} & \textbf{ST2} & \textbf{ST3} & \textbf{GR1} & \textbf{GR2} & \textbf{GR3} & \textbf{Error(\%)} & \textbf{Energy(J)} \\
% & 6 & 14 & 14 & 32 & 32 & 32  
% & 8 & 8 & 12 & 32 & 32 & 32   
% & 14 & 6 & 14 & 16 & 32 & 32 

% 6_12_14_8_32_32 0.919 42.457
% 6_8_8_16_24_32 0.917 31.865
% 6_10_14_4_32_32 0.915 31.152
% 14_14_12_4_16_32 0.914 34.876
% 12_14_14_4_16_32 0.913 33.726
% 14_12_12_4_16_32 0.911 31.246
      \hline 
%       \multirow{6}{*}{Baselines} 
      CondenseNet 122 & 20 & 20 & 20 & 8 & 16 & 32 & 4.48 & 129.37\\
      CondenseNet 110 & 18 & 18 & 18 & 8 & 16 & 32 & 4.63 & 108.74\\
      CondenseNet  98 & 16 & 16 & 16 & 8 & 16 & 32 & 4.83 & 88.73\\
      CondenseNet  86 & 14 & 14 & 14 & 8 & 16 & 32 & 5.06 & 71.98\\
      CondenseNet  74 & 12 & 12 & 12 & 8 & 16 & 32 & 5.28 & 56.35\\
      CondenseNet  50 & 8 & 8 & 8 & 8 & 16 & 32 & 6.22 & 40.35\\
      \hline
      
      \hline 
      \multirow{4}{*}{CondenseNet-MONAS}
      & 6 & 14 & 14 & 32 & 32 & 32 & 4.34 & 92.16\\
      & 8 & 8 & 12 & 32 & 32 & 32 & 4.56 & 79.93\\
      %& 14 & 6 & 14 & 16 & 32 & 32 &  & 74.98\\
      & 6 & 12 & 14 & 8 & 32 & 32 & 5.07 & 42.46\\
	  & 14 & 14 & 12 & 4 & 16 & 32 & 5.6 & 34.88 \\
      \hline
      \multicolumn{9}{l}{ST: Stage, GR: Growth}\\
      \multicolumn{9}{l}{Energy: Energy cost every 1000 inferences}
    \end{tabular}
    \caption{\textbf{MONAS models and CondenseNet Baselines}}
    \label{tab:hparams}
  \end{center}
\end{table*}

% \begin{figure}[h!]
% % \centering
% \includegraphics[width=0.5\textwidth]{FIG/condensenet_0_75_tree.pdf}
% \caption{\condensenet search probability path }
% \label{fig:condensenet_tree_0.75}
% \end{figure}

% when we sample 10000 times for the final probability outputs of the experiment in Fig.~\ref{fig:condensenet_0.75}, completing a graph of weighted paths in Fig.~\ref{fig:condensenet_tree_0.75}. We can observed that the component our method select most frequently is the \textit{growth3=32}, which means the \textit{growth} value for the 3rd dense block.
